# Supplementary material for: Dynamic Camera Poses and Where to Find Them
Source: arXiv:2504.17788 source file (2025-04-24)
Supplement: Supplementary file 1 [file panda70m.tex]

\begin{table*}
\resizebox{\ifdim\width>\linewidth \linewidth \else \width \fi}{!}{

\begin{tabular}{l c c c c c c c c c} \toprule
  & \multicolumn{5}{c}{All 90 Estimable Videos (Identity if Fail)} & \multicolumn{4}{c}{52 Videos: All Succeed Only} \\
 & \% Vids. & \multicolumn{4}{c}{Mean Per-Video Sampson Error, 720p} & \multicolumn{4}{c}{Mean Per-Video Sampson Error, 720p} \\
\textit{Baselines} & Registered$\uparrow$ & $\%<15 $Pix$\uparrow$ & $\%<30$ Pix$\uparrow$ & $\%<60$ Pix$\uparrow$ & Mean$\downarrow$ & $\%<15$ Pix$\uparrow$ & $\%<30$ Pix$\uparrow$ & $\%<60$ Pix$\uparrow$ & Mean$\downarrow$ \\
\midrule
DROID-SLAM~\cite{teed2021droid} & 100. & 87.8 & 94.4 & 98.9 & 11.0 & 90.4 & 96.2 & 100. & 6.78  \\
DUSt3R~\cite{wang2023dust3r} & 100. & 16.7 & 50.0 & 84.4 & 45.5 & 19.2 & 59.6 & 92.3 & 30.0 \\
MonST3R~\cite{zhang2024monst3r} & 100. & 84.4 & 91.1 & 98.9 & 9.89 & 86.5 & 92.3 & 98.1 & 9.73 \\
COLMAP~\cite{schonberger2016structure} & 82.2 & 67.8 & 73.3 & 90.0 & 25.2 & 86.5 & 94.2 & 98.1 & 8.76 \\
COLMAP+Mask~\cite{schonberger2016structure} & 67.8 & 66.7 & 82.2 & 88.9 & 28.4 & 90.4 & 100. & 100. & 5.52 \\
ParticleSfM~\cite{zhao2022particlesfm} & 92.2 & 80.0 & 90.0 & 96.7 & 10.2 & 90.4 & 96.2 & 98.1 & 6.63 \\ 
Ours & 95.6 & 92.2 & 98.9 & 100. & 5.60 & 98.1 & 100. & 100. & 3.61 \\ 
\bottomrule
\end{tabular}
}
\caption{\textbf{Pose + intrinsics estimation on Panda-Test.}
Linear Sampson Error on 10K image pairs, by video, normalized to 720p. Uses pose + intrinsics from method. Static methods DUSt3R and COLMAP struggle faced with dynamics; DROID-SLAM lacks precision but errors tend to be within 60 pixels. 
ParticleSfM registers more videos than COLMAP+Mask but both fall short of Ours in registration, precision and average error on both all (left) and fully-registered videos (right). MonST3R predicts all frames leading to competitive performance across all videos; on videos all methods register Ours outperforms.}
\label{tab:panda}
\end{table*}
